# Supplementary material for: Spontaneously gapped ground state in suspended bilayer graphene
Source: arXiv:1104.3816 source file (2011-06-24)
Supplement: Supplementary file 1 [file Freitag_supplemental.pdf]

# Supplementary Information

## Spontaneously gapped ground state in suspended bilayer graphene

F. Freitag, J. Trbovic, M. Weiss, and C. Schönenberger

Department of Physics, University of Basel, Klingelbergstr. 82, CH-4056 Basel, Switzerland

### Contact resistance determined from QHE

We extract the contact resistance $R_c$ in the following way: The conductance $G$ is plotted as measured and each identifiable Hall plateau in the conductance is assigned to the next higher allowed filling factor $\nu$. For example, a plateau at $G = 0.9\ e^2/h$ would be set to $\nu = 1$. Then $G$ is converted into resistance and plotted against $1/\nu$, as shown in Fig. S1 for sample B2 at 1.5 K. A linear fit is made and the intercept at $\nu \to \infty$, or $1/\nu \to 0$, is $R_c$. This contact resistance is assumed to be purely classical and largely independent of the charge carrier density in the system or the applied perpendicular magnetic field.

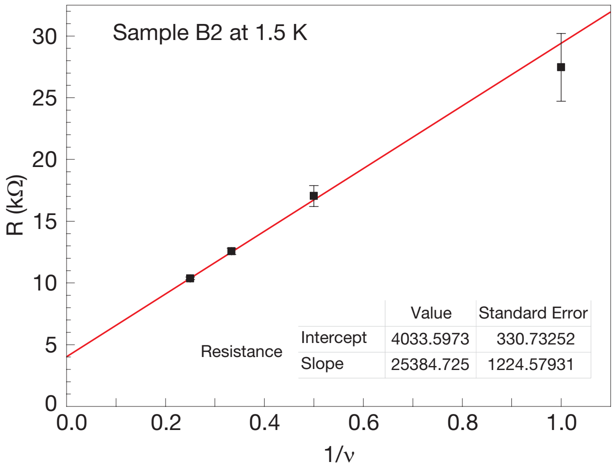


Fig. S 1: **Extraction of $\mathbf{R_c}$.** Plot of the resistance of the Hall plateaus against the inverse of the filling facor $\nu$. The line is a linear fit of the data and its offset at $1/\nu \to 0$ yields the two-terminal contact resistance of $R_c \approx 4$ kΩ. The error bars mark the read-out error.

### Gap in the $\nu = 0$ state in sample B1

The appearance of a highly resistive state with magnetic field $B > B_{crit}$ for sample B1 tuned to the charge-neutrality point (CNP) suggests a transition into a $\nu = 0$ quantum Hall state. This situation can occur because of the lifting of the zero energy Landau level (LL). After the lifting the Fermi energy $E_F$, corresponding to the charge neutral case, will be positioned in between the two LLs at energy $E^+$ and $E^- = -E^+$. This leads to the quantization of the Hall conductance $\sigma_{xy} = \nu e^2/h$ with filling factor $\nu = 0$ in this case, hence, $\sigma_{xy} = 0$. At the same time the dissipative conductance $\sigma_{xx}$ tends to zero, displaying a thermally activated dependence according to $\sigma_{xx} \propto exp(-\Delta E/2k_BT)$, where $\Delta E = E^+ - E^-$ is the activation energy. For the measured electrical resistance $R$ we then expect the following dependence:

$$R = R_0 e^{\Delta E/2k_BT}. \qquad (1)$$

In an electron system with massive electrons (effective mass $m^*$), as is the case for bilayer graphene, adjacent Landau levels are expected to be spaced by the energy $\Delta E = \hbar\omega_c$, where $\omega_c = eB/m^*$ is the cyclotron frequency. The dependence of $ln(R)$ on $B$ should therefore display

a linear dependence on the magnetic field $B$, which is indeed seen in Fig. S2 for magnetic fields above the critical field $B_{crit}$. In addition, and in agreement with thermal activation, the slope increases with decreasing temperature $T$. Assuming $\Delta E = \hbar\omega_c$ and fitting the measurements to the prediction, yields $m^* = 0.1 \pm 0.01\, m_e$, which is roughly three times the theoretical value of $m^* \approx 0.033\ m_e$ [1]. Although the result of a slightly increased mass maybe plausible, we stress that the analysis in this from is incorrect. Assuming $\Delta E = \hbar\omega_c$ means accepting the result from the non-interacting Fermi gas. The non-interacting model provides, however, no mechanism for the lifting of the zero-energy Landau level. Hence, it is better to talk of an apparent energy gap $\Delta E$ which is proportional to $B$ and amounts to $\approx 13\,\mathrm{K/T}$ (Kelvin per Tesla) or $1.1\,\mathrm{meV/T}$. Note, that this number is much larger than the Zeeman splitting, only amounting to $\sim 0.7\,\mathrm{K/T}$.

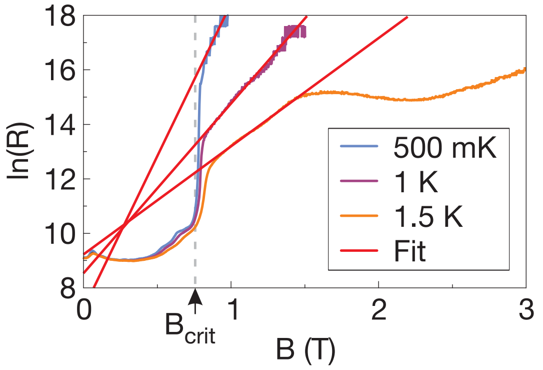


Fig. S 2: **Activated behaviour in $\nu = 0$ state in sample B1.** Log-lin plot of the resistance $R$ of B1 near the CNP as a function of the magnetic field $B$ for different temperatures. Above $B_{crit}$, bilayer graphene enters the insulating $\nu = 0$ state. In the activated regime, $log(R)$ is inversely proportional to temperature and proportional to $B$.

**Absence of a phase transition close to the CNP in sample B2 in low magnetic field**
In Fig. S3a, a colour scale plot of the conductance $G$ of sample B2 is shown as a function of gate voltage $V_g$ and magnetic field $B$. We have looked carefully into the region of low magnetic field close to the CNP to rule out any additional phase transitions. Based on a peak that occurred in $G$ at around 40 mT Weitz *et al.* suggested the appearance of yet another phase [2]. For sample B2, no peak in $G$ is discernible in the measurements shown in Fig. S3. $G$ is constant with the exception of fluctuations.

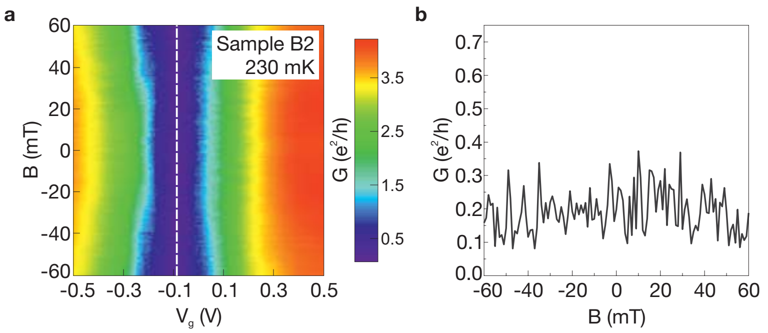


Fig. S 3: **Absence of a phase transition close to the CNP in B2.** **a**, Colour scale of the conductance $G$ of sample B2 as a function of gate voltage $V_g$ and magnetic field $B$. There is no transition into another phase with magnetic field, which would manifest as a notable change in conductance. **b**, Line profile taken at the CNP, as indicated by the dashed line in **a**.

**Comparison of bilayer graphene B2 samples**
We investigated three samples of type B2. In all of them a gap opens at zero field, as shown in Fig. S4. Whereas sample B2a and B2b are different devices, B2c is B2b after thermal cycling, exposure to air and subsequent current annealing. We would like to stress, that B2c did not show a gap before the current annealing and attribute this to disorder introduced by adsorbates from the air.

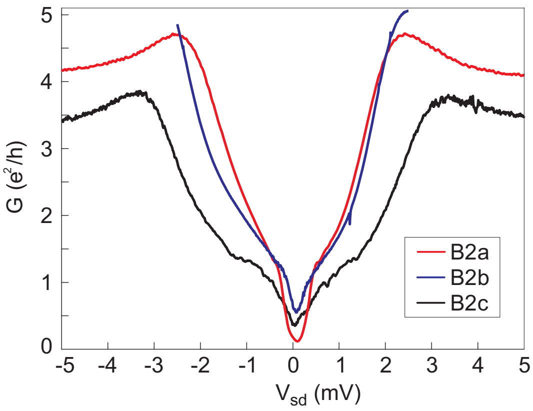


Fig. S 4: **Comparison of gaps of type B2 samples.** The conductance $G$ as a function of $V_{sd}$ at 230 mK. In all three samples, a larger gap of size $\Delta = 2 - 3\,\text{meV}$ and a smaller one of size $\delta \approx 0.2 - 0.5\,\text{meV}$ are clearly visible.

## References


1. Das Sarma, S., Adam, S., Hwang, E. H. & Rossi, E. Electronic transport in two dimensional graphene. *arXiv:1003.4731v2* (2010).

2. Weitz, R. T., Allen, M. T., Feldman, B. E., Martin, J. & Yacoby, A. Broken-Symmetry States in Doubly Gated Suspended Bilayer Graphene. *Science* **330,** 812–816 (2010).
